# Supplementary material for: Out-of-equilibrium collective oscillation as phonon condensation in a model protein
Source: arXiv:1705.07975 source file (2018-07-23)
Supplement: Supplementary file 1 [file supplementary-final.pdf]

# Supplementary Information on "Out-of-equilibrium collective oscillation as phonon condensation in a model protein"

**by I. Nardecchia et al.**

## I. PROPERTIES OF THE LIOUVILLIAN FOR THE CLASSICAL MODEL

In order to derive the classical rate equations, we now apply the method described in the main paper to the model described by the Hamiltonian in Eq.(27). We introduce a *multiplicative* operator for scalar functions $\widehat{\mathcal{M}}_{f(\{(J_\omega,\theta_\omega)\}_{\omega\in\mathcal{I}_\mathcal{S}})}$ as

$$\widehat{\mathcal{M}}_{f(\{(J_\omega,\theta_\omega)\}_{\omega\in\mathcal{I}_\mathcal{S}})}\,|\psi\rangle = f(\{(J_\omega,\theta_\omega)\}_{\omega\in\mathcal{I}_\mathcal{S}})\psi = |f(\{(J_\omega,\theta_\omega)\}_{\omega\in\mathcal{I}_\mathcal{S}})\psi\rangle \tag{1}$$

and *derivative* operators with respect to the angular variables $\widehat{D}_{\theta_\omega}$, and with respect to the action variables $\widehat{D}_{J_\omega}$ as

$$\widehat{D}_{J_\omega}\,|\psi\rangle = -\imath\partial_{J_\omega} f \qquad \widehat{D}_{\theta_\omega}\,|\psi\rangle = -\imath\partial_{\theta_\omega} f\ . \tag{2}$$

The commutation rules for such operators are obviously given by

$$\begin{aligned}
&\left[\widehat{\mathcal{M}}_{f(\{(J_\omega,\theta_\omega)\}_{\omega\in\mathcal{I}_\mathcal{S}})}, \widehat{\mathcal{M}}_{g(\{(J_\omega,\theta_\omega)\}_{\omega\in\mathcal{I}_\mathcal{S}})}\right] = 0 && \text{(commutativity of product of functions)}\\
&\left[\widehat{D}_{J_{\omega_i}}, \widehat{D}_{\theta_{\omega_j}}\right] = \left[\widehat{D}_{J_{\omega_i}}, \widehat{D}_{J_{\omega_j}}\right] = \left[\widehat{D}_{\theta_{\omega_i}}, \widehat{D}_{\theta_{\omega_j}}\right] = 0 && \text{(Schwarz Theorem for } C^2 \text{ functions)}\\
&\left[\widehat{D}_{J_{\omega_i}}, \widehat{\mathcal{M}}_{f(\{(J_\omega,\theta_\omega)\}_{\omega\in\mathcal{I}_\mathcal{S}})}\right] = -\imath\widehat{\mathcal{M}}_{\partial_{J_{\omega_i}} f(\{(J_\omega,\theta_\omega)\}_{\omega\in\mathcal{I}_\mathcal{S}})} && \text{(Leibniz rule of derivation)}\\
&\left[\widehat{D}_{\theta_{\omega_i}}, \widehat{\mathcal{M}}_{f(\{(J_\omega,\theta_\omega)\}_{\omega\in\mathcal{I}_\mathcal{S}})}\right] = -\imath\widehat{\mathcal{M}}_{\partial_{\theta_{\omega_i}} f(\{(J_\omega,\theta_\omega)\}_{\omega\in\mathcal{I}_\mathcal{S}})}\ .
\end{aligned} \tag{3}$$

in particular, from the general formulas (3) one gets

$$\begin{aligned}
&\left[\widehat{D}_{J_{\omega_i}}, \widehat{\mathcal{M}}_{J^q_{\omega_j}}\right] = -\imath q\widehat{\mathcal{M}}_{J^{q-1}_{\omega_i}}\delta_{ij} \qquad \omega_i,\omega_j\in\mathcal{I}_\mathcal{S} \quad q\in\mathbb{Z}\\
&\left[\widehat{D}_{\boldsymbol{\alpha}\cdot\boldsymbol{\theta}}, \widehat{\mathcal{M}}_{\exp[\imath\boldsymbol{\beta}\cdot\boldsymbol{\theta}]}\right] = (\boldsymbol{\alpha}\cdot\boldsymbol{\beta})\ \widehat{\mathcal{M}}_{\exp[\imath\boldsymbol{\beta}\cdot\boldsymbol{\theta}]} \qquad \boldsymbol{\alpha}\cdot\boldsymbol{\beta} = \sum_{\omega_i\in\mathcal{I}_\mathcal{S}} \alpha_{\omega_i}\beta_{\omega_i}\\
&\left[\widehat{D}_{\boldsymbol{\alpha}\cdot\boldsymbol{\theta}}, \widehat{\mathcal{M}}_{\cos[\boldsymbol{\beta}\cdot\boldsymbol{\theta}]}\right] = \imath(\boldsymbol{\alpha}\cdot\boldsymbol{\beta})\ \widehat{\mathcal{M}}_{\sin[\boldsymbol{\beta}\cdot\boldsymbol{\theta}]} \qquad \left[\widehat{D}_{\boldsymbol{\alpha}\cdot\boldsymbol{\theta}}, \widehat{\mathcal{M}}_{\sin[\boldsymbol{\beta}\cdot\boldsymbol{\theta}]}\right] = -\imath(\boldsymbol{\alpha}\cdot\boldsymbol{\beta})\ \widehat{\mathcal{M}}_{\cos[\boldsymbol{\beta}\cdot\boldsymbol{\theta}]}
\end{aligned} \tag{4}$$

where

$$\widehat{D}_{\boldsymbol{\alpha}\cdot\boldsymbol{\theta}} = -\imath\sum_{\omega\in\mathcal{I}_\mathcal{S}} \alpha_\omega\widehat{\partial}_{\theta_\omega} \qquad \alpha_\omega\in\mathbb{R},. \tag{5}$$

With this definition, and for the system under consideration, it follows that the free Liouville operator $\widehat{\mathcal{L}}_{H_0}$ can be rewritten as

$$\widehat{\mathcal{L}}_{H_0} = -\imath\sum_{\omega\in\mathcal{I}_\mathcal{S}} \omega\widehat{\partial}_{\theta_\omega} = \widehat{D}_{\boldsymbol{\omega}\cdot\boldsymbol{\theta}}\ . \tag{6}$$

The Liouville interaction operator is the sum of four contributions

$$\widehat{\mathcal{L}}_{H_{int}}(t) = \widehat{\mathcal{L}}_{H_{sys-bth}}(t) + \widehat{\mathcal{L}}_{H_{sys-src}}(t) + \widehat{\mathcal{L}}_{H_{sys-bth-src}}(t) + \widehat{\mathcal{L}}_{H_{IntQ}}(t) \tag{7}$$

where the explicit time dependence takes into account the adiabatic switching off of the interaction at $t = +\infty$; this is obtained by the introduction of a term of the form $\exp[-\lambda t]$ where $\lambda > 0$ is the inverse time scale during which the interaction is assumed to be active.

The term $\widehat{\mathcal{L}}_{H_{sys-bth}}(t)$ and $\widehat{\mathcal{L}}_{H_{sys-src}}(t)$ describes the linear interactions among the normal modes of the macromolecule, of the thermal bath, and of the external source of energy, which are respectively given by

$$\widehat{\mathcal{L}}_{H_{sys-bth}}(t) = \sum_{\omega \in \mathcal{I}_{sys}} \sum_{\Omega \in \mathcal{I}_{bth}} \exp(-\lambda t)\, \eta_{\omega\Omega} \Big[ \widehat{\mathcal{M}}_{J_\omega^{1/2}} \widehat{\mathcal{M}}_{J_\Omega^{1/2}} \widehat{\mathcal{M}}_{\sin(\theta_\omega - \theta_\Omega)} \left( \widehat{D}_{J_\omega} - \widehat{D}_{J_\Omega} \right) + \\ + \frac{1}{2} \widehat{\mathcal{M}}_{\cos(\theta_\omega - \theta_\Omega)} \left( \widehat{\mathcal{M}}_{J_\omega^{-1/2}} \widehat{\mathcal{M}}_{J_\Omega^{1/2}} \widehat{D}_{\theta_\omega} + \widehat{\mathcal{M}}_{J_\omega^{1/2}} \widehat{\mathcal{M}}_{J_\Omega^{-1/2}} \widehat{D}_{\theta_\Omega} \right) \Big] \tag{8}$$

and

$$\widehat{\mathcal{L}}_{H_{sys-src}}(t) = \sum_{\omega \in \mathcal{I}_{sys}} \sum_{\Omega' \in \mathcal{I}_{src}} \exp(-\lambda t)\, \eta_{\omega\Omega'} \Big[ \widehat{\mathcal{M}}_{J_\omega^{1/2}} \widehat{\mathcal{M}}_{J_{\Omega'}^{1/2}} \widehat{\mathcal{M}}_{\sin(\theta_\omega - \theta_{\Omega'})} \left( \widehat{D}_{J_\omega} - \widehat{D}_{J_{\Omega'}} \right) + \\ + \frac{1}{2} \widehat{\mathcal{M}}_{\cos\left(\theta_\omega - \theta_{\Omega'}\right)} \left( \widehat{\mathcal{M}}_{J_\omega^{-1/2}} \widehat{\mathcal{M}}_{J_{\Omega'}^{1/2}} \widehat{D}_{\theta_\omega} + \widehat{\mathcal{M}}_{J_\omega^{1/2}} \widehat{\mathcal{M}}_{J_{\Omega'}^{-1/2}} \widehat{D}_{\theta_{\Omega'}} \right) \Big] \; . \tag{9}$$

The Liouvillian operator associated with the non linear interaction term between the normal modes of the main system with the thermal bath is given by

$$\widehat{\mathcal{L}}_{H_{sys-bth-sys}}(t) = \\ = \sum_{\omega, \omega_i \in \mathcal{I}_{sys}} \sum_{\Omega_{bth} \in \mathcal{I}_{bth}} \exp(-\lambda t) \Big\{ \widehat{\mathcal{M}}_{J_\omega^{1/2}} \widehat{\mathcal{M}}_{J_{\omega_i}^{1/2}} \widehat{\mathcal{M}}_{J_\Omega^{1/2}} \Big[ \chi_{\omega\omega_i\Omega} \widehat{\mathcal{M}}_{\sin\left(\theta_\omega + \theta_\Omega - \theta_{\omega_i}\right)} \left( \widehat{D}_{J_\omega} + \widehat{D}_{J_\Omega} \right) + \\ + \chi_{\omega_i\omega\Omega} \widehat{\mathcal{M}}_{\sin\left(\theta_{\theta_\omega - \omega_i} - \theta_\Omega\right)} \widehat{D}_{J_\omega} \Big] + \frac{1}{2} \widehat{\mathcal{M}}_{J_\omega^{-1/2}} \widehat{\mathcal{M}}_{J_{\omega_i}^{1/2}} \widehat{\mathcal{M}}_{J_\Omega^{1/2}} \Big[ \chi_{\omega\omega_i\Omega} \widehat{\mathcal{M}}_{\cos\left(\theta_\omega + \theta_\Omega - \theta_{\omega_i}\right)} + \\ \chi_{\omega_i\omega\Omega} \widehat{\mathcal{M}}_{\cos\left(\theta_{\omega_i} + \theta_\Omega - \theta_\omega\right)} \Big] \widehat{D}_{\theta_\omega} + \frac{1}{2} \widehat{\mathcal{M}}_{J_\omega^{1/2}} \widehat{\mathcal{M}}_{J_{\omega_i}^{1/2}} \widehat{\mathcal{M}}_{J_\Omega^{-1/2}} \widehat{\mathcal{M}}_{\cos\left(\theta_\omega + \theta_\Omega - \theta_{\omega_i}\right)} \widehat{D}_{\theta_\Omega} \Big\} \tag{10}$$

Under the simplifying hypothesis that the coefficients $\kappa_{(n)\omega_i\omega_j\omega_k\omega_l}$ are symmetric with respect to the exchange of symbols then the terms representing quartic anharmonic interactions

among the normal modes are given by

$$\widehat{\mathcal{L}}_{H_{intQ}}(t) = \sum_{\omega,\omega_i,\omega_j,\omega_k \in \mathcal{I}_{sys}} \exp\left(-\lambda t\right) \Bigg\{ \widehat{\mathcal{M}}_{J_\omega^{1/2}} \widehat{\mathcal{M}}_{J_{\omega_i}^{1/2}} \widehat{\mathcal{M}}_{J_{\omega_j}^{1/2}} \widehat{\mathcal{M}}_{J_{\omega_k}^{1/2}} \Bigg[ 4\kappa_{(1)\omega\omega_i\omega_j\omega_k} \widehat{\mathcal{M}}_{\sin(\omega+\omega_i-\omega_j-\omega_k)} +$$
$$+ \kappa_{(2)\omega\omega_i\omega_j\omega_k} \left( 3\widehat{\mathcal{M}}_{\sin\left(\theta_\omega+\theta_{\omega_i}+\theta_{\omega_j}+\theta_{\omega_k}\right)} + \widehat{\mathcal{M}}_{\sin\left(\theta_\omega-\theta_{\omega_i}-\theta_{\omega_j}-\theta_{\omega_k}\right)} \right) +$$
$$+ 4\kappa_{(3)\omega\omega_i\omega_j\omega_k} \widehat{\mathcal{M}}_{\sin\left(\theta_\omega+\theta_{\omega_i}+\theta_{\omega_j}+\theta_{\omega_k}\right)} \Bigg] \widehat{D}_{J_\omega} + \frac{1}{2} \widehat{\mathcal{M}}_{J_\omega^{1/2}} \widehat{\mathcal{M}}_{J_{\omega_i}^{1/2}} \widehat{\mathcal{M}}_{J_{\omega_j}^{1/2}} \widehat{\mathcal{M}}_{J_{\omega_k}^{1/2}} \Bigg[$$
$$4\kappa_{(1)\omega\omega_i\omega_j\omega_k} \widehat{\mathcal{M}}_{\cos\left(\theta_\omega+\theta_{\omega_i}-\theta_{\omega_j}-\theta_{\omega_k}\right)} + \kappa_{(2)\omega\omega_i\omega_j\omega_k} \left( 3\widehat{\mathcal{M}}_{\cos\left(\theta_\omega+\theta_{\omega_i}+\theta_{\omega_j}-\theta_{\omega_k}\right)} + \widehat{\mathcal{M}}_{\sin\left(\theta_\omega-\theta_{\omega_i}-\theta\omega_j-\theta\omega_k\right)} \right) +$$
$$+ 4k_{(3)\omega\omega_i\omega_j\omega_k} \widehat{\mathcal{M}}_{\sin\left(\theta_\omega+\theta_{\omega_i}+\theta_{\omega_j}+\theta_{\omega_k}\right)} \Bigg] \widehat{D}_{\theta_\omega} \quad . \tag{11}$$

The particular form of the Liouville operator imposes some restriction on the domain of the $L^2$ functions on phase space that have to be considered. The Liouvillian operator for the model that has been introduced is invariant under angle translation by multiples of $2\pi$

$$\exp[\imath 2\pi \widehat{D}_{\mathbf{k}\cdot\boldsymbol{\theta}}] \mathcal{L}_H(\boldsymbol{\theta}, t) \exp[-\imath 2\pi \widehat{D}_{\mathbf{k}\cdot\boldsymbol{\theta}}] = \mathcal{L}_H(\boldsymbol{\theta} + 2\pi\mathbf{k}, t) = \mathcal{L}_H(\boldsymbol{\theta}, t) \qquad \mathbf{k} \in \mathbb{Z}^{N_{tot}} \tag{12}$$

where $N_{tot}$ is the total number of normal modes of the main system, of the thermal bath and of the external source. The property (12) implies that we can limit the domain of the operator to the space of $2\pi$-periodic functions with respect to the angle variables: hence any function in the domain of the operator can be written in terms of Fourier series

$$\psi(\{(J_\omega, \theta_\omega)\}_{\omega\in\mathcal{I}_\mathcal{S}}, t) = \sum_{\mathbf{k}\in\mathbb{Z}^{N_{tot}}} \frac{1}{(2\pi)^{N_{tot}}/2} \phi_{\mathbf{k}} \left(\{(J_\omega\}_{\omega\in\mathcal{I}_\mathcal{S}}, t\right) \exp\left[-\imath \mathbf{k}\cdot\boldsymbol{\theta}\right] \tag{13}$$

with the normalization condition

$$\sum_{\mathbf{k}\in\mathbb{Z}^{N_{tot}}} \|\phi_{\mathbf{k}} \left(\{(J_\omega\}_{\omega\in\mathcal{I}_\mathcal{S}}, t\right)\|^2 = 1\,. \tag{14}$$

In order to verify that the considered Liouville operator is hermitian, it is sufficient to prove that the following operator, depending only on a pair of action-angle variables, is hermitian

$$\widehat{\mathcal{L}}_{test} = \widehat{\mathcal{M}}_{J_\omega^{k/2}} \widehat{\mathcal{M}}_{\sin(\theta_\omega+\delta)} \widehat{D}_{J_\omega} + \left(\mathbb{I} + \frac{1}{2}\widehat{\mathcal{M}}_{J_\omega^{k/2-1}} \widehat{\mathcal{M}}_{\cos(\theta_\omega+\delta)}\right) \widehat{D}_{\theta_\omega} \qquad \text{with} \quad k \geq 1 \tag{15}$$

so that

$$
\begin{aligned}
&\left\langle g \middle| \widehat{\mathcal{L}}_{test} f \right\rangle = \\
&= -\imath \int_0^{2\pi} \mathrm{d}\theta_\omega \int_0^{+\infty} \mathrm{d}J_\omega \; g^* \left[ J_\omega^{k/2} \sin(\theta+\delta) \frac{\partial f}{\partial J} + \left( \frac{k}{2} J_\omega^{k/2-1} \cos(\theta_\omega+\delta) + 1 \right) \frac{\partial f}{\partial \theta_\omega} \right] = \\
&= -\imath \int_0^{2\pi} \mathrm{d}\theta_\omega J_\omega^{k/2} \sin(\theta_\omega+\delta)\, g^* f \Bigg|_{J=0}^{J=+\infty} + \imath \int_0^{2\pi} \mathrm{d}\theta_\omega \int_0^{+\infty} \mathrm{d}J_\omega \; \sin(\theta_\omega+\delta)\, J_\omega^{k/2} \frac{\partial g^*}{\partial_{J_\omega}} + \\
&+ \imath \frac{k}{2} \int_0^{2\pi} \mathrm{d}\theta_\omega \int_0^{+\infty} \mathrm{d}J_\omega \sin(\theta_\omega+\delta)\, g^* f - \imath \frac{k}{2} \int_0^{+\infty} \mathrm{d}J_\omega \; \left( \cos(\theta_\omega+\delta)\, J_\omega^{k/2-1} + 1 \right) g^* f \Bigg|_{\theta=0}^{\theta=2\pi} + \\
&+ \imath \frac{k}{2} \int_0^{2\pi} \mathrm{d}\theta_\omega \int_0^{+\infty} \mathrm{d}J_\omega \; \left( \cos(\theta_\omega+\delta)\, J_\omega^{k/2-1} + 1 \right) \frac{\partial g^*}{\partial \theta_\omega} f + \\
&- \imath \frac{k}{2} \int_0^{2\pi} \mathrm{d}\theta_\omega \int_0^{+\infty} \mathrm{d}J_\omega \; \sin(\theta_\omega+\delta)\, J_\omega^{k/2-1} g^* f = \\
&= \left\langle \widehat{\mathcal{L}}_{test} g \middle| f \right\rangle - \imath \frac{k}{2} \int_0^{+\infty} \mathrm{d}J_\omega \; \left( \cos(\theta_\omega+\delta)\, J_\omega^{k/2-1} + 1 \right) g^* f \Bigg|_{\theta=0}^{\theta=2\pi} + \\
&- \imath \int_0^{2\pi} \mathrm{d}\theta_\omega J_\omega^{k/2} \sin(\theta_\omega+\delta)\, g^* f \Bigg|_{J=0}^{J=+\infty} \quad .
\end{aligned}
\tag{16}
$$

So, if we consider a domain of functions in $L^2([0,2\pi]\times[0,+\infty))$ such that they are periodic in the angle variables and such that for both $f, g$ it is

$$
\lim_{J_\omega \longrightarrow 0} J_\omega^{1/4} \phi(\{J_\omega\}_{\omega\in\mathcal{I}_\mathcal{S}}) = 0 \;, \tag{17}
$$

then the operator $\widehat{\mathcal{L}}_{test}$ is hermitian, and, consequently, the Liouville operator associated with the model under consideration is hermitian.

We remark that if we consider the Fourier representation of the amplitude functions $\psi$ as in Eq.(13) and we make the hypothesis that the only non zero component is $\phi_{\mathbf{0}}(\{J_\omega\}_{\omega\in\mathcal{I}_\mathcal{S}}, t)$, then it can be verified that the square root of the normalized Boltzmann distribution for independent harmonic oscillators at equilibrium

$$
\phi_{\mathrm{Bol}}(J_\omega, t) = \sqrt{\frac{k_B T}{\omega}} \exp\left[ -\frac{\omega J_\omega}{2 k_B T} \right] \tag{18}
$$

satisfies the condition in Eq.(17).

In what follows we assume that the amplitude of the test function $|\psi(t)\rangle_S$ in Schrödinger

representation has the form

$$|\psi(t)\rangle_S = \phi_{\mathbf{0}}(\{J_\omega\}_{\omega\in\mathcal{I}_\mathcal{S}}) = \prod_{\omega\in\mathcal{I}_{sys}} \phi(J_\omega, t) \prod_{\Omega\in\mathcal{I}_{bth}} \phi_{\mathrm{Bol}}(J_\Omega) \prod_{\Omega'\in\mathcal{I}_{src}} \phi_{\mathrm{Bol}}(J_{\Omega'})\,. \tag{19}$$

This assumption on the form of the states we are interested in accounts for several physical approximations. The independence on the angular variables (as $\phi_{\mathbf{k}}(\{J_\omega\}_{J_\omega\in\mathcal{I}_\mathcal{S}}, t) = 0$ for $\mathbf{k}\neq\mathbf{0}$) can be interpreted as a mutual independence of the angular variables. Moreover, the factorization of $|\psi(t)\rangle_S$ in terms of the actions of single harmonic oscillators of the thermal baths (both sink and external source ), according to Boltzmann time-independent distribution functions, is a possible formalization of a thermal bath whose degrees of freedom have their own statistics and are not influenced by the dynamics. Finally, the factorization of the distribution function of the normal modes of the system stems from the assumption that the action variables of the main system are statistically independent, that is

$$\left\langle \prod_{\omega\in\mathcal{I}_\mathcal{S}} J_\omega^{k_\omega} \right\rangle \approx \prod_{\omega\in\mathcal{I}_\mathcal{S}} \left\langle J_\omega^{k_\omega}\right\rangle \ . \tag{20}$$

### A. Derivation of the rate equations for the expectation values of the actions $J_{\omega_i}$

We first notice that for an operator $\widehat{\mathcal{A}}_I(t)$ in Interaction Picture one has

$$\frac{\mathrm{d}\widehat{\mathcal{A}}_I(t)}{\mathrm{d}t} = \exp\left(\imath t\widehat{\mathcal{L}}_{H_0}\right)\left[\widehat{\mathcal{A}}_S(t), \widehat{\mathcal{L}}_{H_0}\right]\exp\left(-\imath t\widehat{\mathcal{L}}_{H_0}\right) \tag{21}$$

so that the time dependence of an operator $\widehat{\mathcal{A}}_I(t)$ is obtained only through multiplicative operators for functions of angular variables only, $\widehat{\mathcal{M}}_{f(\{\theta_\omega\}_{\omega\in\mathcal{I}_\mathcal{S}})}$; in the Liouville operator associated to the Hamiltonian in Eq.(27) of the main paper, these functions have the general form

$$\begin{aligned}\widehat{\mathcal{M}}_{\cos(\mathbf{k}\cdot\boldsymbol{\theta})} &= \frac{\widehat{\mathcal{M}}_{\exp(\imath\mathbf{k}\cdot\boldsymbol{\theta})} + \widehat{\mathcal{M}}_{\exp(-\imath\mathbf{k}\cdot\boldsymbol{\theta})}}{2}\\ \widehat{\mathcal{M}}_{\sin(\mathbf{k}\cdot\boldsymbol{\theta})} &= \frac{\widehat{\mathcal{M}}_{\exp(\imath\mathbf{k}\cdot\boldsymbol{\theta})} - \widehat{\mathcal{M}}_{\exp(-\imath\mathbf{k}\cdot\boldsymbol{\theta})}}{2\imath}\,.\end{aligned} \tag{22}$$

with $\mathbf{k}\in\mathbb{R}^{N_{Tot}}$. As the following differential equation holds

$$\begin{aligned}\frac{\mathrm{d}\left(\widehat{\mathcal{M}}_{\pm\imath\exp(\pm\imath\mathbf{k}\cdot\boldsymbol{\theta})}\right)_I}{\mathrm{d}t} &= \frac{\mathrm{d}}{\mathrm{d}t}\left[\exp\left(\imath t\widehat{\mathcal{L}}_{H_0}\right)\left(\widehat{\mathcal{M}}_{\pm\imath\exp(\pm\imath\mathbf{k}\cdot\boldsymbol{\theta})}\right)_S\exp\left(-\imath t\widehat{\mathcal{L}}_{H_0}\right)\right] =\\ &= \pm\imath\left(\mathbf{k}\cdot\boldsymbol{\omega}t\right)\left(\widehat{\mathcal{M}}_{\pm\imath\exp(\pm\imath\mathbf{k}\cdot\boldsymbol{\theta})}\right)_I(t)\end{aligned} \tag{23}$$

it follows that

$$\left(\widehat{\mathcal{M}}_{\pm\imath\exp(\pm\imath\mathbf{k}\cdot\boldsymbol{\theta})}\right)_I(t) = \exp\left(\pm\imath\mathbf{k}\cdot\boldsymbol{\omega}\right)\left(\widehat{\mathcal{M}}_{\pm\exp(\pm\imath\mathbf{k}\cdot\boldsymbol{\theta})}\right) \tag{24}$$

and consequently

$$\begin{aligned}\left(\widehat{\mathcal{M}}_{\cos(\mathbf{k}\cdot\boldsymbol{\theta})}\right)_I(t) &= \widehat{\mathcal{M}}_{\cos(\mathbf{k}\cdot(\boldsymbol{\theta}+\boldsymbol{\omega}t))}\\ \left(\widehat{\mathcal{M}}_{\sin(\mathbf{k}\cdot\boldsymbol{\theta})}\right)_I(t) &= \widehat{\mathcal{M}}_{\sin(\mathbf{k}\cdot(\boldsymbol{\theta}+\boldsymbol{\omega}t))}\,.\end{aligned} \tag{25}$$

Now we have all the elements to derive the rate equations from Eq.(46) of the main paper.

### 1. *Linear term of $\widehat{\mathcal{L}}_{H_{Int}}$ in Eq.(46)*

We start considering the contribution of the first order term in $\widehat{\mathcal{L}}_{H_{Int}}$ to the right hand side of the rate equations (46). This term is given by the expectation value of the commutator of $\widehat{\mathcal{L}}_{H_{Int}}$ with the multiplication operator for the action variables $J_{\omega_i}$ (in Interaction Picture) computed on the initial unperturbed state $|\psi_0(-\infty)\rangle$ .
Using the commutation rules in Eq.(4) and Eqs.(25) it follows

$$\begin{aligned}&\left(\left[\hat{\mathcal{L}}_H,\hat{\mathcal{M}}_{J_{\omega_i}}\right]\right)_I(t) = (-\imath)\exp\left(-\lambda t\right)\left(\sum_{\Omega\in\mathcal{I}_{sys}}\eta_{\omega_i\Omega}\widehat{\mathcal{M}}_{J_{\omega_i}^{1/2}}\widehat{\mathcal{M}}_{J_{\Omega}^{1/2}}\widehat{\mathcal{M}}_{\sin\left[\theta_{\omega_i}-\theta_\Omega+(\omega_i+\Omega)t\right]}+\right.\\
&+\sum_{\Omega'\in\mathcal{I}_{src}}\xi_{\omega_i\Omega'}\widehat{\mathcal{M}}_{J_{\omega_i}^{1/2}}\widehat{\mathcal{M}}_{J_{\Omega'}^{1/2}}\widehat{\mathcal{M}}_{\sin\left[\theta_{\omega_i}-\theta_{\Omega'}+(\omega_i-\Omega')t\right]}+\\
&+\sum_{\omega_j\in\mathcal{I}_{sys}}\sum_{\Omega\in\mathcal{I}_{bth}}\widehat{\mathcal{M}}_{J_{\omega_i}^{1/2}}\widehat{\mathcal{M}}_{J_{\omega_j}^{1/2}}\widehat{\mathcal{M}}_{J_{\Omega}^{1/2}}\left(\chi_{\omega_i\omega_j\Omega}\widehat{\mathcal{M}}_{\sin\left[\theta_{\omega_i}+\theta_\Omega-\theta_{\omega_j}+(\omega_i+\Omega-\omega_j)t\right]}+\right.\\
&\left.-\chi_{\omega_j\omega_i\Omega}\widehat{\mathcal{M}}_{\sin\left[\theta_{\omega_i}-\theta_{\omega_j}-\theta_\Omega+(\omega_i-\omega_j-\Omega)t\right]}\right)+\\
&+\sum_{\omega_j,\omega_k,\omega_l\in\mathcal{I}_{sys}}\widehat{\mathcal{M}}_{J_{\omega_i}^{1/2}}\widehat{\mathcal{M}}_{J_{\omega_j}^{1/2}}\widehat{\mathcal{M}}_{J_{\omega_k}^{1/2}}\widehat{\mathcal{M}}_{J_{\omega_l}^{1/2}}\left[4\kappa_{(1)\omega_i\omega_j\omega_k\omega_l}\widehat{\mathcal{M}}_{\sin\left[\theta_{\omega_i}+\theta_{\omega_j}-\theta_{\omega_k}-\theta_{\omega_l}+(\omega_i+\omega_j-\omega_k-\omega_l)t\right]}+\right.\\
&+\kappa^{(2)}_{\omega_i\omega_j\omega_k\omega_l}\left(\widehat{\mathcal{M}}_{\sin\left[\theta_{\omega_i}-\theta_{\omega_j}-\theta_{\omega_k}-\theta_{\omega_l}+(\omega_i-\omega_j-\omega_k-\omega_l)t\right]}+3\widehat{\mathcal{M}}_{\sin\left[\theta_{\omega_i}-\theta_{\omega_j}-\theta_{\omega_k}-\theta_{\omega_l}+(\omega_i-\omega_j-\omega_k-\omega_l)t\right]}\right)+\\
&\left.+\kappa^{(3)}_{A_iA_jA_kA_l}\widehat{\mathcal{M}}_{\sin\left[\theta_{\omega_i}+\theta_{\omega_j}+\theta_{\omega_k}+\theta_{\omega_l}+(\omega_i-\omega_j-\omega_k-\omega_l)t\right]}\right]\,.\end{aligned} \tag{26}$$

Note that all terms depend linearly on sine functions of the angular variables. The expectation value of these terms, computed on the state $|\psi_0\rangle$ defined in Eq.(19), gives a vanishing contribution because these trigonometric functions are averaged on the interval

$[0;2\pi]$. This means that the lowest order contribution to the rate equations for the $\langle J_{\omega_i}\rangle$ comes from the quadratic term in $\widehat{\mathcal{L}}_{H_{Int}}$.

### 2. Second order term in $\widehat{\mathcal{L}}_{H_{Int}}$ in Eq.(46)

The second order term with respect to $\widehat{\mathcal{L}}_{H_{Int}}$ in the right hand side of Eq. (46) contains quadratic terms of trigonometric functions of the angular variables, thus their expectation values computed on $|\psi_0\rangle$ of Eq.(19) are non vanishing .
The general form for these terms is given by

$$\left\langle \widehat{\mathcal{M}}_{J_\omega} \right\rangle = \sum_{(i),(ii)\in IdxSet} \langle\psi_0| \int_0^t \mathrm{d}t' \left[ \left( \left[ \widehat{\mathcal{L}}_{H_{(i)}}, \widehat{\mathcal{M}}_{J_\omega} \right] \right)_I (t), \left( \widehat{\mathcal{L}}_{H_{(ii)}} \right)_I (t') \right] |\psi_0\rangle \tag{27}$$

where $IdxSet = \{sys-bth,\, sys-src,\, sys-src-sys,\, intQ(1),\, intQ(2),\, intQ(3)\}$ is the set of indices labelling the different terms entering the Liouville interaction operator; this means that *a priori* one has to compute 36 different terms. However, thanks to the form of the state $|\psi_0(t)\rangle$, some of these terms can be eliminated by parity arguments. In fact, only those terms which depend on even powers of trigonometric functions do not vanish when averaged; this happens only when the same indices in $IdxSet$ are considered.
As an example of how the computation proceeds, let us follow the detailed derivation of the contribution to the rate equations given by the term describing linear interactions among the bath and the main system.
First, consider the operator at the right hand side of (27) where $(i) = (ii) = sys-bth$, at time $t>0$, expressed in Interaction Picture

$$\begin{aligned}
&\int_0^t \left[ \left( \left[ \widehat{\mathcal{L}}_{H_{sys-bth}}, \widehat{\mathcal{M}}_{J_{\omega_i}} \right] \right)_I (t), \left( \widehat{\mathcal{L}}_{sys-bth} \right)_I (t') \right] \mathrm{d}t' = \\
&= \frac{1}{2} \sum_{\omega\in\tilde{\mathcal{I}}_{sys}} \sum_{\Omega,\tilde{\Omega}\in\mathcal{I}_{bth}} \int_0^t \exp(-\lambda t) \exp(-\lambda t')\, \eta_{\omega_i\tilde{\Omega}} \eta_{\omega\Omega} \widehat{\mathcal{M}}_{J_\omega^{1/2}} \widehat{\mathcal{M}}_{J_\Omega^{1/2}} \Bigg[ \Bigg( \widehat{\mathcal{M}}_{J_{\omega_i}^{-1/2}} \widehat{\mathcal{M}}_{J_{\tilde{\Omega}}^{1/2}} \delta_{\omega,\omega_i} + \\
&- \widehat{\mathcal{M}}_{J_{\omega_i}^{1/2}} \widehat{\mathcal{M}}_{J_{\tilde{\Omega}}^{-1/2}} \delta_{\Omega,\tilde{\Omega}} \Bigg) \widehat{\mathcal{M}}_{\sin\left[\theta_{\omega_i}-\theta_{\tilde{\Omega}}+\left(\omega_i-\tilde{\Omega}\right)t\right]} \widehat{\mathcal{M}}_{\sin[\theta_\omega-\theta_\Omega+(\omega-\Omega)t']} + \Bigg( \widehat{\mathcal{M}}_{J_{\omega_i}^{-1/2}} \widehat{\mathcal{M}}_{J_{\tilde{\Omega}}^{1/2}} \delta_{\omega,\omega_i} + \\
&- \widehat{\mathcal{M}}_{J_{\omega_i}^{1/2}} \widehat{\mathcal{M}}_{J_{\tilde{\Omega}}^{-1/2}} \delta_{\Omega,\tilde{\Omega}} \Bigg) \widehat{\mathcal{M}}_{\cos\left[\theta_{\omega_i}-\theta_{\tilde{\Omega}}+(\omega_i-\tilde{\Omega})t\right]} \widehat{\mathcal{M}}_{\cos[\theta_\omega-\theta_\Omega+(\omega-\Omega)t']} \Bigg) \Bigg] \mathrm{d}t' \ ,
\end{aligned} \tag{28}$$

then, integrating on $t'$, and taking the limit $\lambda \to 0$, one obtains

$$\int_0^t \left[\left(\left[\widehat{\mathcal{L}}_{H_{sys-bth}}, \widehat{\mathcal{M}}_{J_{\omega_i}}\right]\right)_I(t), \left(\widehat{\mathcal{L}}_{sys-bth}\right)_I(t')\right] \mathrm{d}t' =$$

$$= \frac{1}{2} \sum_{\omega \in \tilde{\mathcal{I}}_{sys}} \sum_{\Omega, \tilde{\Omega} \in \mathcal{I}_{bth}} \eta_{\omega_i \tilde{\Omega}} \eta_{\omega \Omega} \, \widehat{\mathcal{M}}_{J_\omega^{1/2}} \widehat{\mathcal{M}}_{J_\Omega^{1/2}} \frac{\sin\left(\frac{(\omega-\Omega)t}{2}\right)}{(\omega-\Omega)} \left[\left(\widehat{\mathcal{M}}_{J_{\omega_i}^{-1/2}} \widehat{\mathcal{M}}_{J_{\tilde{\Omega}}^{1/2}} \delta_{\omega,\omega_i} + \right.\right.$$

$$\left. - \widehat{\mathcal{M}}_{J_{\omega_i}^{1/2}} \widehat{\mathcal{M}}_{J_{\tilde{\Omega}}^{-1/2}} \delta_{\Omega,\tilde{\Omega}}\right) \left(\widehat{\mathcal{M}}_{\cos\left[\theta_\omega - \theta_\Omega - \theta_{\omega_i} + \theta_{\tilde{\Omega}} + \left(\omega - \Omega - \frac{\omega_i - \tilde{\Omega}}{2}\right)t\right]} + \right. \tag{29}$$

$$\left. - \widehat{\mathcal{M}}_{\cos\left[\theta_\omega - \theta_\Omega + \theta_{\omega_i} - \theta_{\tilde{\Omega}} + \left(\omega - \Omega + \frac{\omega_i - \tilde{\Omega}}{2}\right)t\right]}\right) + \left(\widehat{\mathcal{M}}_{J_{\omega_i}^{-1/2}} \widehat{\mathcal{M}}_{J_{\tilde{\Omega}}^{1/2}} \delta_{\omega,\omega_i} - \widehat{\mathcal{M}}_{J_{\omega_i}^{1/2}} \widehat{\mathcal{M}}_{J_{\tilde{\Omega}}^{-1/2}} \delta_{\Omega,\tilde{\Omega}}\right)$$

$$\left(\widehat{\mathcal{M}}_{\cos\left[\theta_\omega - \theta_\Omega - \theta_{\omega_i} + \theta_{\tilde{\Omega}} + \left(\omega - \Omega - \frac{\omega_i - \tilde{\Omega}}{2}\right)t\right]} + \widehat{\mathcal{M}}_{\cos\left[\theta_\omega - \theta_\Omega + \theta_{\omega_i} - \theta_{\tilde{\Omega}} + \left(\omega - \Omega + \frac{\omega_i - \tilde{\Omega}}{2}\right)t\right]}\right),$$

when the expectation value of this term is computed on $|\psi_0\rangle$, the non vanishing terms are those for which $\omega \in \mathcal{I}_{sys}$ and $\Omega \in \mathcal{I}_{bth}$ are such that the trigonometric functions in (29) do not depend any longer on the angular variables, that is, such that $\omega = \omega_i$ and $\Omega = \tilde{\Omega}$. In this way non vanishing averages on the angular variables are obtained, and the final average of Eq. (29) reads

$$\langle\psi_0| \int_0^t \left[\left(\left[\widehat{\mathcal{L}}_{H_{sys-bth}}, \widehat{\mathcal{M}}_{J_{\omega_i}}\right]\right)_I(t), \left(\widehat{\mathcal{L}}_{sys-bth}\right)_I(t')\right] \mathrm{d}t' \, |\psi_0\rangle =$$

$$= \sum_{\tilde{\Omega} \in \mathcal{I}_{bth}} \left(\frac{\pi}{2} \eta^2_{\omega_i \tilde{\Omega}}\right) \frac{\sin\left[\left(\omega - \tilde{\Omega}\right)t\right]}{\pi\left(\omega - \tilde{\Omega}\right)} \left(\left\langle \widehat{\mathcal{M}}_{J_{\tilde{\Omega}}} \right\rangle - \left\langle \widehat{\mathcal{M}}_{J_{\omega_i}} \right\rangle\right) \tag{30}$$

where the brackets in the above expression refer to the averaging on the actions variables. A consequence of the form of the $|\psi_0\rangle$ function, defined in Eq.(19), is that the expectation values of the action variables of the heath bath are

$$\left\langle \widehat{\mathcal{M}}_{J_{\tilde{\Omega}}} \right\rangle = \frac{k_B T_B}{\tilde{\Omega}} \,. \tag{31}$$

In the limit in which the thermal bath is modelled by a continuous set of normal modes, the coefficients $\eta^2_{\omega\tilde{\Omega}}$ turn into a distribution function of the frequencies of the modes of the thermal bath, that is, $\eta^2_{\omega\tilde{\Omega}} \to \eta^2_\omega(\tilde{\Omega})$, with the obvious replacement $\sum_{\tilde{\Omega} \in \mathcal{I}_{bth}} \to \int_0^{+\infty} \mathrm{d}\tilde{\Omega}$. As we are interested in the behaviour of the system for long times, that is $t \gg \max_{\omega \in \mathcal{I}_{sys}, \tilde{\Omega} \in \mathcal{I}_{bth}} |\tilde{\Omega} - \omega|^{-1}$, the following approximation can be done

$$\frac{\sin\left[\left(\omega - \tilde{\Omega}\right)t\right]}{\pi\left(\omega - \tilde{\Omega}\right)} \longrightarrow \delta(\omega - \tilde{\Omega}) \,. \tag{32}$$

Finally, the averages over the action variables evaluated at $t_0 = 0$ are assumed to be a good approximation at any time $t$, since in the spirit of perturbation theory, $|\psi_0(t)\rangle \approx |\psi_0(t_0)\rangle$, thus

$$\left\langle \widehat{\mathcal{M}}_{J_{\omega_i}} \right\rangle = \int_0^{+\infty} J_{\omega_i} \|\phi_0(J_{\omega_i};0)\|^2 \approx \int_0^{+\infty} J_{\omega_i} \|\phi_0(J_{\omega_i};t)\|^2 = \left\langle \widehat{\mathcal{M}}_{J_{\omega_i}} \right\rangle (t) \ , \tag{33}$$

which is, by the way, the same approximation made by Wu and Austin in their derivation of the Fröhlich quantum rate equations [1].

The final result for the linear main system-thermal bath interaction is

$$\langle\psi_0| \int_0^t \left[ \left( \left[ \widehat{\mathcal{L}}_{H_{sys-bth}}, \widehat{\mathcal{M}}_{J_{\omega_i}} \right] \right)_I (t), \left( \widehat{\mathcal{L}}_{sys-bth} \right)_I (t') \right] \mathrm{d}t' \, |\psi_0\rangle = \left( \frac{\pi}{2} \eta^2_{\omega_i}(\omega_i) \right) \left[ \frac{k_B T_B}{\omega_i} - \langle J_{\omega_i} \rangle \right]$$
$$= b_{\omega_i} \left[ \frac{k_B T_B}{\omega_i} - \langle J_{\omega_i} \rangle \right] \tag{34}$$

where $b_{\omega_i} = \pi \eta^2_{\omega_i}(\omega_i)/2\omega_i$ . A similar derivation is worked out for the linear coupling between the main system and the thermal bath at higher temperature $T_P$, which models the source of energy pumping into the system, yielding

$$\langle\psi_0| \int_0^t \left[ \left( \left[ \widehat{\mathcal{L}}_{H_{sys-src}}, \widehat{\mathcal{M}}_{J_{\omega_i}} \right] \right)_I (t), \left( \widehat{\mathcal{L}}_{sys-src} \right)_I (t') \right] |\psi_0\rangle \ \mathrm{d}t' = \frac{\pi \xi^2_{\omega_i(\omega_i)}}{2} \left( \frac{k_B T_P}{\omega_i} - \langle J_{\omega_i} \rangle \right)$$
$$\simeq \frac{\pi \xi^2_{\omega_{A_i} \omega_{A_i}}}{2} \frac{k_B T_P}{\omega_{A_i}} = s_{\omega_i} \tag{35}$$

where it has been assumed that $\langle J_{\omega_i} \rangle (t) \ll \dfrac{k_B T_P}{\omega_i}$. This approximation corresponds to the physical request of a continuous, non-negative, and time independent energy injection into each normal mode $\omega_i$ at some corresponding rate $s_{\omega_i}$.

The contribution to the rate equations coming from the non linear interaction between the main system and the thermal bath is more tricky and finally reads as

$$\langle\psi_0| \int_0^t \left[ \left( \left[ \widehat{\mathcal{L}}_{H_{sys-bth-sys}}, \widehat{\mathcal{M}}_{J_{\omega_i}} \right] \right)_I (t), \left( \widehat{\mathcal{L}}_{H_{sys-bth-sys}} \right)_I (t') \right] |\psi_0\rangle \ \mathrm{d}t'$$
$$= \sum_{\omega \in \mathcal{I}_{sys}} \frac{\pi \chi^2_{\omega_i \omega}(|\omega - \omega_i|)}{2} \left[ \frac{k_B T_B}{|\omega - \omega_i|} \left( \langle J_\omega \rangle - \langle J_{\omega_i} \rangle \right) + \mathrm{sgn}(\omega - \omega_i) \langle J_{\omega_i} J_\omega \rangle \right]$$
$$\simeq \sum_{\omega_i \in \mathcal{I}_{sys}} \frac{\pi \chi^2_{\omega_i \omega}(|\omega - \omega_i|)}{2} \left[ \frac{k_B T_B}{|\omega - \omega_i|} \left( \langle J_\omega \rangle - \langle J_{\omega_i} \rangle \right) + \mathrm{sgn}(\omega - \omega_i) \langle J_{\omega_i} \rangle \langle J_\omega \rangle \right] \tag{36}$$

where the factorization $\langle J_{\omega_i} J_\omega \rangle \simeq \langle J_{\omega_i} \rangle \langle J_\omega \rangle$, in the last term of the r.h.s. of the equation just above, implies the assumption that the correlations between the actions of the normal

modes are negligible. Introducing the coefficients

$$c_{\omega\omega_i} = \frac{\pi k_B T_B \chi^2_{\omega_i\omega}(|\omega - \omega_i|)}{2|\omega - \omega_i|} \tag{37}$$

equation (36) simplifies to

$$\begin{aligned}&\langle\psi_0| \int_0^t \left[\left(\left[\widehat{\mathcal{L}}_{H_{H_{sys-bth-sys}}}, \widehat{\mathcal{M}}_{J_{\omega_i}}\right]\right)_I(t), \left(\widehat{\mathcal{L}}_{H_{sys-bth-sys}}\right)_I(t')\right] |\psi_0\rangle \; \mathrm{d}t' = \\ &= \sum_{\omega_A \in \mathcal{I}_{sys}} c_{\omega\omega_i} \left[ (\langle J_\omega\rangle - \langle J_{\omega_i}\rangle) + \frac{(\omega - \omega_i)}{k_B T_B} \langle J_{\omega_i}\rangle \langle J_\omega\rangle \right].\end{aligned} \tag{38}$$

Previously, while modelling the heath bath with a continuum of modes, we replaced $\sin\left[(\omega_i - \Omega)t\right] / \left[\pi(\omega_i - \Omega)\right]$ with a a $\delta$-distribution, whereas if the number of vibrational modes of the main system (macromolecule) is supposed to be finite or countably infinite, then the sinc function is better replaced by

$$\frac{\sin\left[\Delta\omega_{(A)intQ}(\omega_i)t\right]}{\pi\Delta\omega_{(A)intQ}(\omega_i)} \approx \begin{cases} 0 & \text{when} \quad \Delta\omega_{(A)intQ}(\omega_i) \neq 0 \\ \dfrac{1}{\delta\omega_{sys}} & \text{when} \quad \Delta\omega_{(i)} = 0 \end{cases} \tag{39}$$

where $\delta\omega_{sys} = \min \omega_j, \omega_k \in \mathcal{I}_{sys}(|\omega_j - \omega_k|)$ is the spectral resolution of the main system, and

$$\begin{aligned}\Delta\omega_{(1)intQ}(\omega_i) &= \omega_i + \omega_j - \omega_k - \omega_l \qquad \Delta\omega_{(2,i)intQ}(\omega_i) = \omega_i - \omega_j - \omega_k - \omega_l \\ \Delta\omega_{(2,ii)intQ} &= \omega_i + \omega_j + \omega_k - \omega_l \qquad \Delta\omega_{(3)intQ} = \omega_i + \omega_j + \omega_k + \omega_l\end{aligned} \tag{40}$$

are the resonance conditions for the different quartic terms. Note that under this approximation the contribution given by the terms $\widehat{\mathcal{L}}_{(3)intQ}$ vanish as $\omega > 0$. The remaining quartic terms respectively yield

$$\begin{aligned}&\langle\psi_0| \int_0^t \left[\left(\left[\widehat{\mathcal{L}}_{H_{(1)intQ}}, \widehat{\mathcal{M}}_{J_{\omega_i}}\right]\right)_I(t), \left(\widehat{\mathcal{L}}_{H_{(1)intQ}}\right)_I(t')\right] |\psi_0\rangle \; \mathrm{d}t' = \\ &= \sum_{\substack{\omega_j,\omega_k,\omega_l \in \mathcal{I}_{sys} \\ \omega_i+\omega_j-\omega_k-\omega_l=0}} \frac{16\pi\kappa^2_{(1)\omega_i\omega_j\omega_k\omega_l}}{\delta\omega_{sys}} \langle J_{\omega_l}\rangle \Big( \langle J_{\omega_j}\rangle \langle J_{\omega_k}\rangle + \langle J_{\omega_i}\rangle \langle J_{\omega_k}\rangle - 2\langle J_{\omega_i}\rangle \langle J_{\omega_j}\rangle \Big)\end{aligned} \tag{41}$$

and

$$\begin{aligned}&\langle\psi_0| \int_0^t \left[\left(\left[\widehat{\mathcal{L}}_{H_{(2)intQ}}, \widehat{\mathcal{M}}_{J_{\omega_i}}\right]\right)_I(t), \left(\widehat{\mathcal{L}}_{H_{(2)intQ}}\right)_I(t')\right] |\psi_0\rangle \; \mathrm{d}t' = \\ &= \frac{3\pi}{\delta\omega_{sys}} \Bigg[ \sum_{\substack{\omega_j\omega_k\omega_l \in \mathcal{I}_{sys} \\ \omega_i+\omega_j+\omega_k-\omega_l=0}} 3\kappa^2_{(2)\omega_i\omega_j\omega_k\omega_l} \langle J_{\omega_l}\rangle \Big( \langle J_{\omega_j}\rangle \langle J_{\omega_k}\rangle + 2\langle J_{\omega_i}\rangle \langle J_{\omega_k}\rangle - \langle J_{\omega_i}\rangle \langle J_{\omega_j}\rangle \Big) + \\ &+ \sum_{\substack{\omega_j\omega_k\omega_l \in \mathcal{I}_{sys} \\ \omega_i-\omega_j-\omega_k-\omega_l=0}} \kappa^2_{(2)\omega_i\omega_j\omega_k\omega_l} \langle J_{\omega_l}\rangle \langle J_{\omega_k}\rangle \Big( \langle J_{\omega_j}\rangle - 3\langle J_{\omega_i}\rangle \Big) \Bigg].\end{aligned} \tag{42}$$

Putting together all the above derived terms, one finally gets the following rate equations

$$\frac{\mathrm{d}\langle J_{\omega_i}\rangle}{\mathrm{d}t} = s_{\omega_i} + b_{\omega_i}\left[\frac{k_B T_B}{\omega_i} - \langle J_{\omega_i}\rangle\right] + \sum_{\substack{\omega_j\in\mathcal{I}_{sys}\\ \omega_j\neq\omega_i}} c_{\omega_i\omega_j}\left[\left(\langle J_{\omega_j}\rangle - \langle J_{\omega_i}\rangle\right) + \frac{\omega_j-\omega_i}{k_B T_B}\langle J_{\omega_i}\rangle\langle J_{\omega_j}\rangle\right] +$$
$$+ \sum_{\substack{\omega_j,\omega_k,\omega_l\in\mathcal{I}_{sys}\\ \omega_i+\omega_j-\omega_k-\omega_l=0}} \frac{16\pi\kappa^2_{(1)\omega_i\omega_j\omega_k\omega_l}}{\delta\omega_{sys}}\langle J_{\omega_l}\rangle\left(\langle J_{\omega_j}\rangle\langle J_{\omega_k}\rangle + \langle J_{\omega_i}\rangle\langle J_{\omega_k}\rangle - 2\langle J_{\omega_i}\rangle\langle J_{\omega_j}\rangle\right)$$
$$+ \frac{3\pi}{\delta\omega_{sys}}\left[\sum_{\substack{\omega_j\omega_k\omega_l\in\mathcal{I}_{sys}\\ \omega_i+\omega_j+\omega_k-\omega_l=0}} 3\kappa^2_{(2)\omega_i\omega_j\omega_k\omega_l}\langle J_{\omega_l}\rangle\left(\langle J_{\omega_j}\rangle\langle J_{\omega_k}\rangle + 2\langle J_{\omega_i}\rangle\langle J_{\omega_k}\rangle - \langle J_{\omega_i}\rangle\langle J_{\omega_j}\rangle\right) +\right.$$
$$\left. + \sum_{\substack{\omega_j\omega_k\omega_l\in\mathcal{I}_{sys}\\ \omega_i-\omega_j-\omega_k-\omega_l=0}} \kappa^2_{(2)\omega_i\omega_j\omega_k\omega_l}\langle J_{\omega_l}\rangle\langle J_{\omega_k}\rangle\left(\langle J_{\omega_j}\rangle - 3\langle J_{\omega_i}\rangle\right)\right]. \tag{43}$$

which have been given in the main text of this paper, and which are in the form of a nonlinear dynamical system describing the time evolution of the expectation values of the actions, that is, of the amplitudes of the normal modes of a generically modelled macromolecule.


[1] T.M. Wu and S. Austin, Bose-Einstein condensation in biological systems. J. Theor. Biology **71**, 209 - 214 (1978).
